# Supplementary material for: Robust Multiple Kernel k-means Clustering using Min-Max Optimization
Source: arXiv:1803.02458 source file (2019-09-10)
Supplement: Supplementary file 1 [file MultiViewScenarios.tex]

\begin{figure}[!ht]
	\centering
	\includegraphics[width=\textwidth]{figure/scenAllpaper.pdf}
	\caption{\textbf{Multi-view Scenarios.} (A) Scenario A is composed of a complete view and a partial view. (B) Scenario B is composed of two partial views. (C) Scenario C is composed of two partial views and a `noise' view. In our simulation experiments, we modified each scenario by (1) adding numbers of noise variables ($N_{noise} = 1, 2, \cdots$), or (2) adding numbers of redundant pairs to the first view ($N_{redunPairs} = 1, 2, \cdots$) as well as increasing correlation level between the first pair and the redundant pairs ($cor = 0.45, 0.72, 0.90, 0.97, 1$). Each of the noise variables are independently sampled from Gaussian distribution with zero-mean and unit-variance. The samples in the heatmaps are ordered by their true cluster index. %The redundant pairs are generated to be correlated with the first pair with $r^2 \approx 0.7$.
	}\label{fig:multiviewscenAll}\label{fig:multiviewscenA}\label{fig:multiviewscenB}\label{fig:multiviewscenC}
\end{figure}
\bigskip ~~~
